# Supplementary material for: Accelerating the Registration of Image Sequences by Spatio-temporal Multilevel Strategies
Source: arXiv:2001.06613 source file (2020-01-18)
Supplement: Supplementary file 1 [file supplementary.tex]

\section{Supplementary Material}

\subsection{Discretization}

We perform numerical integration using Trapezoidal rule 
\begin{align*}
    & \int_a^b g(t) \ dt \approx (t_1 - a) g(t_1) \\ & + \sum_{i=2}^{N} \frac{(t_i - t_{i-1})}{2} (g(t_{i-1}) + g(t_i)) + (b - t_N) g(t_N).
\end{align*}
This is also a mid-point quadrature rule if sampling points have uniform spacing between them and function values are defined at the center of the grid.

\subsection{Convergence Proofs}

Prove that $\|w_{l+1} - w_{N}\| \leq \|w_{l} - w_{N}\|$ where $N$ is the last stage in the multilevel framework.

\begin{figure}
    \centering
    \begin{tikzpicture}[
    squarednode/.style={rectangle, draw=black, very thick}, scale = 0.8]
    %Nodes
    \node[]                 (initialN1)                               {$\sY_{N_1}$};
    \node[squarednode]      (prolongN1)       [right=0.5 cm of initialN1]    {$P\sY_{N_1}$};
    \node[]                 (initialN2)       [right=0.5 cm of prolongN1]    {$\sY^0_{N_2}$};
    \node[squarednode]      (optimize)        [right=0.5 cm of initialN2]    {solve \eqref{simmeasdisc}};
    \node[]                 (outputN2)        [right=0.5 cm of optimize]     {$\sY_{N_2}$};
    \node[squarednode]      (prolongN2)       [right=0.5 cm of outputN2]     {$P\sY_{N_2}$};

    %Lines
    \draw[->] (initialN1.east) -- (prolongN1.west);
    \draw[->] (prolongN1.east) -- (initialN2.west);
    \draw[->] (initialN2.east) -- (optimize.west);
    \draw[->] (optimize.east) --  (outputN2.west);
    \draw[->] (outputN2.east) --  (prolongN2.west);
    
    \end{tikzpicture}
    \caption{Parameters flow at a temporal level $l^t$}
    \label{fig:ytflow}
\end{figure}

We introduce an index set $\sI_K = \{1,\dots,K\}$ where $K \in \posn$. Let $\sS_N$ be an N-element subset of $\sI_K$ such that $\sS_N \cap \sS_{K-N} = \emptyset$. Let $\sY_N = (y_{t_n})_{n \in \sS_N}$ be a sequence of transformation fields such that $ \sY_K= (y_{t_1},\dots,y_{t_K})$.

We wish to find out conditions such that the following inequality holds:
\begin{align}
    D[P\sY_{N_1}] \leq D[P\sY_{N_2}] 
\end{align}
where $P$ represents the temporal prolongation operation and $N_1 \leq N_2 \leq K$. Please see Fig.~\ref{fig:ytflow}.

We divide the sequence $\sY_K$ into two subsequences $\sY_{N}$ and $\sY_{K-N}$. Following this, we can decompose similarity measure \eqref{simmeasdisc} as
\begin{align}\label{simdecom}
    D[\sY_K] &= \sum_{(i,j) \in \sS_N} w_{ij} \rho_{ij}^2 + \sum_{(i,j) \in \sI_K\setminus\sS_{N}} w_{ij} \rho_{ij}^2 \nonumber \\ 
    & + \sum_{i \in \sS_{N}, j \in \sI_K\setminus\sS_{N}} w_{ij} \rho_{ij}^2 \nonumber \\
           &= D[\sY_{N}] + D[\sY_{K-N}] + D_M[\sY_{K}]
\end{align}
where $D_M$ has mixed terms from the two subsequences.

note:(union of subsequences - not a rigorous mathematical notation )

Considering $\sY^0_K = P\sY_{N_1} = \sY^0_{N_2} \cup \sY^0_{K - N_2}$ and following \eqref{simdecom}, we can write
\begin{align}\label{eqy0}
    D[P\sY_{N_1}] = D[\sY^0_{N_2}] + D[\sY^0_{K-N_2}] + D_M[\sY^0_{K}].
\end{align}

Considering $\sY^*_K = P\sY_{N_2} = \sY_{N_2} \cup \sY^*_{K - N_2}$ and following \eqref{simdecom}, we can write
\begin{align}\label{eqy1}
    D[P\sY_{N_2}] = D[\sY_{N_2}] + D[\sY^*_{K-N_2}] + D_M[\sY^*_{K}].
\end{align}

Considering $\sY_K = \sY_{N_2} \cup \sY^0_{K - N_2}$ and following \eqref{simdecom}, we can write
\begin{align}\label{eqy2}
    D[\sY_K] = D[\sY_{N_2}] + D[\sY^0_{K-N_2}] + D_M[\sY_{K}].
\end{align}

\subsection{Derivatives}

Let $y = (y_{t_1}, \dots, y_{t_K})$ be a sequence of transformation fields for a given image sequence $ T = (\Tc_{t_1}, \dots, \Tc_{t_K})$. We define a feature matrix $F = [f_{t_1}, \dots, f_{t_K}]$ where $f_{t_k} = f(\Tc_{t_k}(y_{t_k}))$ and $f$ is a feature function, e.g., NCC, NGF. The correlation coefficient between two feature functions reads
\begin{align}
    \rho_{ij} = \langle f_{t_i}, f_{t_j} \rangle
\end{align}
where the usual normalization factors are considered as a part of the feature function $f$.

The similarity measure \eqref{simmeasdisc} after spatial discretization reads
\begin{align}
    D^h(y) &= h_d \sum_{i=1}^{K} \sum_{j=1}^{K} w_i w_j \rho_{ij}^2 = h_d \| W^{\circ 1/2} \circ C \|_F^2
\end{align}
and its first derivative with respect to $y_{t_k}$ is given as
\begin{align}\label{gradDyk}
    \partial_{y_{t_k}} D^h(y) &= 4 h_d \sum_{i=1}^{K} w_i w_k \ \rho_{ik} \ f_{t_i}^T \ \nabla_{y_{t_k}} f_{t_k} \nonumber \\
                            &= 4 h_d (W_k \circ C_k) F^T \nabla_{y_{t_k}} f_{t_k}
\end{align}
where $W_k$ and $C_k$ denotes the $k^{th}$ row of the matrix.

\subsection{Stopping Criterion}
At a specific spatial level, stopping rule at each temporal level is
\begin{align}
	\| \sWc_N - (\sWc_N)_{old}\| \leq eps*\| \sWc_K\|
\end{align}
$\| \sWc_K\|$ will be same for each temporal level and it is equal to the estimate computed at the previous spatial level.
